# Supplementary material for: Career Incentives, Risk-Taking, and Sorting Dynamics: Evidence from Top Financial Advisers
Source: arXiv:2503.23763 source file (2025-03-31)
Supplement: Supplementary file 1 [file a_3_2.tex]

%----------------------------------------------------------------
\subsection{%Disparity in Career Concerns and Risk-Taking} 
Human Capital Investment, 
Risk-Taking, 
and 
%Firm Selection
Downward Mobility
}
%----------------------------------------------------------------
\label{app: manager 2}

In this section, we contrast the career trajectories of top managers with those of top advisers. Our analysis examines three dimensions:

B.2.1 Human Capital Investment in Qualification:
We re-estimate the baseline model, replacing “Top Adviser” with “Top Manager” and focusing on the acquisition of the Series 24 exam (required for principal/supervisor roles). Table B.1 shows that, in early career stages (0–4 years), top managers are over twice as likely to obtain the Series 24 exam, and this differential increases to 7.5 times after assuming a management position.

B.2.2 Risk-Taking in Regulatory Actions:
We modify the model to focus on regulatory actions as a measure of risk-taking, controlling for firm size dummies (“Mid/Large”) with small firms as the base category. Table B.2 reveals that, after being in a management position, small-firm top managers are approximately four times more likely to face regulatory actions than average advisers, while top managers in mid- and large-sized firms show considerably lower exposure.

B.2.3 Downward Mobility:
We examine downward mobility using “Revenue” as the measure of firm size. Table B.3 indicates that small-firm top managers experience a significant downward mobility penalty—working at firms over 50% smaller than average advisers before management and moving to new firms 20 times smaller post-management—whereas mid/large-firm top managers consistently work at much larger firms compared to average advisers.
