# Supplementary material for: Career Incentives, Risk-Taking, and Sorting Dynamics: Evidence from Top Financial Advisers
Source: arXiv:2503.23763 source file (2025-03-31)
Supplement: Supplementary file 2 [file a_3_1.tex]

%----------------------------------------------------------------
\subsection{Data for Top Managers}
%----------------------------------------------------------------
\label{app: manager 1}

We construct a sample of top managers—specifically CEOs and CFOs—who have served as financial advisers by merging executive information from Form BD (for FINRA-member firms) and Form ADV (for SEC-member firms) with our adviser–level dataset. This matching is based on unique CRD numbers and job titles. Detailed procedures and matching algorithms are provided in Appendix B.1.
