# Supplementary material for: Career Incentives, Risk-Taking, and Sorting Dynamics: Evidence from Top Financial Advisers
Source: arXiv:2503.23763 source file (2025-03-31)
Supplement: Supplementary file 3 [file a_3_3.tex]

%----------------------------------------------------------------
\subsection{
%	Differences in 
Labour-Market Advantages and Penalty Reduction
} 
%----------------------------------------------------------------
\label{app: manager 3}
We analyze whether top managers enjoy labour-market advantages similar to top advisers. Our analysis focuses on market discipline following regulatory actions. Using the same baseline model (with “Top Manager” replacing “Top Adviser”) and restricting the sample to observations after assuming management positions, Table B.4 shows that top managers are more likely to remain with their firms following a regulatory action—by more than 2.5 times—compared to average advisers. However, no significant penalty reduction is observed for top managers in securing new employment upon exit.
%----------------------------------------------------------------
